# Supplementary material for: PriorBoost: An Adaptive Algorithm for Learning from Aggregate Responses
Source: arXiv:2402.04987 source file (2024-02-07)
Supplement: Supplementary file 1 [file appendix_experiments.tex]

\section{Experiments}
\label{app:experiments}

\todo{Probably delete all of this. Here as a placeholder / backup.}

\subsection{Linear regression}

\paragraph{Plot 1 (left)}
Event-level MSE loss for prior-boosting models.
This is a $d$-dimensional linear regression problem for $d=8$
with $r=256$ rounds. In each round we get $1024$ samples and aggregate responses (given by the oracle and our prior model).
Thus, for each plot there are $262,144$ training data points.
We plot the test lost of each model $\th$ one a separate test set of $262,144$ data points.
We sweep bag sizes over $k \in \{1, 2, 4, 8, 16, 32, 64\}$ starting from a random prior.
The solid lines show the performance on the test loss over time of the ``boosting'' models.
The dashed lines show the test loss if we used all of the training data with random bagging and no prior.

\paragraph{Plot 2 (right)}
Next, we repeat the same experiment as in \Cref{fig:linear_regression_plot_prefix_data_side_by_side} (right), but now in each round we train with all the (aggregate) data seen so far. Notice that data points from earlier round are noisier, hence the learner converges more slowly (as a function of rounds) compared to only uses the newest and most accurate aggregate data.

\begin{figure}[H]
\centering
\includegraphics[width=0.235\textwidth]{figures/experiment-2-1.png}
\includegraphics[width=0.235\textwidth]{figures/experiment-2-2.png}
\includegraphics[width=0.235\textwidth]{figures/experiment-2-3.png}
\includegraphics[width=0.235\textwidth]{figures/experiment-2-4.png}
\caption{Linear regression side-by-side plots (1 and 2).}
\label{fig:linear_regression_plot_prefix_data_side_by_side}
\end{figure}

Tables of the data above (mean of last 10 steps)...

\begin{table}[H]
\caption{Linear regression, MSE}
\label{tab:sample-table-1}
\vskip 0.15in
\begin{center}
\begin{small}
\begin{sc}
\begin{tabular}{rcccr}
\toprule
$k$ & \texttt{one-shot} & \texttt{prefix-boost} & \texttt{prior-boost} \\
\midrule
$1$    & 0.0051 & 0.0051 & 0.0051 \\
$2$    & 1.8336 & 0.0051 & 0.0051 \\
$4$    & 4.1317 & 0.0061 & 0.0051 \\
$8$    & 5.6098 & 0.0365 & 0.0051 \\
$16$   & 6.4352 & 0.1338 & 0.0051 \\
$32$   & 6.8721 & 0.3208 & 0.0054 \\
$64$   & 7.0955 & 0.3221 & 0.0061 \\
\bottomrule
\end{tabular}
\end{sc}
\end{small}
\end{center}
\vskip -0.1in
\end{table}

\begin{table}[H]
\caption{Linear regression, RRE}
\label{tab:sample-table-2}
\vskip 0.15in
\begin{center}
\begin{small}
\begin{sc}
\begin{tabular}{rcccr}
\toprule
$k$ & \texttt{one-shot} & \texttt{prefix-boost} & \texttt{prior-boost} \\
\midrule
$1$    & 0.0001 & 0.0001 & 0.0012 \\
$2$    & 0.4998 & 0.0023 & 0.0011 \\
$4$    & 0.7508 & 0.0122 & 0.0013 \\
$8$    & 0.8749 & 0.0657 & 0.0021 \\
$16$   & 0.9372 & 0.1328 & 0.0033 \\
$32$   & 0.9685 & 0.2079 & 0.0066 \\
$64$   & 0.9841 & 0.2081 & 0.0116 \\
\bottomrule
\end{tabular}
\end{sc}
\end{small}
\end{center}
\vskip -0.1in
\end{table}

\subsection{Logistic regression}

\paragraph{Plot 1 (left)}
Here we sweep over bags of size:
$k \in (1, 2, 4, 8, 16, 32, 64)$.
\todo{Describe rounding. Model always takes 0-1 labels as input (i.e., mean label is rounded --> another source of noise).}

\todo{Hyperparams in appendix}

L2 regularization: $\lambda = 10$

\begin{figure}[H]
\centering
\includegraphics[width=0.235\textwidth]{figures/experiment-3-1.png}
\includegraphics[width=0.235\textwidth]{figures/experiment-3-2.png}
\includegraphics[width=0.235\textwidth]{figures/experiment-3-3.png}
\includegraphics[width=0.235\textwidth]{figures/experiment-3-4.png}
\caption{Logistic regression side-by-side plots (1 and 2).}
\label{fig:logistic_regression_plot_prefix_data_side_by_side}
\end{figure}

Tables of the data above (mean of last 10 steps)...

\begin{table}[H]
\caption{Logistic regression, MSE}
\label{tab:sample-table-3}
\vskip 0.15in
\begin{center}
\begin{small}
\begin{sc}
\begin{tabular}{rcccr}
\toprule
$k$ & \texttt{one-shot} & \texttt{prefix-boost} & \texttt{prior-boost} \\
\midrule
$1$    & 0.1398 & 0.1411 & 0.1415 \\
$2$    & 0.4243 & 0.1426 & 0.1418 \\
$4$    & 0.4882 & 0.1441 & 0.1425 \\
$8$    & 0.5396 & 0.1522 & 0.1438 \\
$16$   & 0.5798 & 0.1651 & 0.1473 \\
$32$   & 0.6107 & 0.2619 & 0.1477 \\
$64$   & 0.6329 & 0.2261 & 0.1464 \\
\bottomrule
\end{tabular}
\end{sc}
\end{small}
\end{center}
\vskip -0.1in
\end{table}

\begin{table}[H]
\caption{Logistic regression, RRE}
\label{tab:sample-table-4}
\vskip 0.15in
\begin{center}
\begin{small}
\begin{sc}
\begin{tabular}{rcccr}
\toprule
$k$ & \texttt{one-shot} & \texttt{prefix-boost} & \texttt{prior-boost} \\
\midrule
$1$    & 0.4142 & 0.4203 & 0.4207 \\
$2$    & 0.8806 & 0.4268 & 0.4216 \\
$4$    & 0.9171 & 0.4294 & 0.4217 \\
$8$    & 0.9417 & 0.4382 & 0.4222 \\
$16$   & 0.9589 & 0.4486 & 0.4248 \\
$32$   & 0.9710 & 0.5193 & 0.4246 \\
$64$   & 0.9792 & 0.4918 & 0.4235 \\
\bottomrule
\end{tabular}
\end{sc}
\end{small}
\end{center}
\vskip -0.1in
\end{table}

\subsection{Label differential privacy}

For fixed value of $\varepsilon$, it is not necessarily better to just use $k=1$ and Laplace noise (i.e., label DP). Instead, bagging and using less random noise can be a better way to achieve $\varepsilon$-DP (i.e., better model quality).

\todo{Table of case study for $\varepsilon = 1$ (different algorithms, bag sizes).}

\begin{table}[H]
\caption{Logistic regression + DP ($\varepsilon = 1$)}
\label{tab:sample-table-3}
\vskip 0.15in
\begin{center}
\begin{small}
\begin{sc}
\begin{tabular}{rcccr}
\toprule
$k$ & \texttt{one-shot} & \texttt{prefix-boost} & \texttt{prior-boost} \\
\midrule
$1$    & 0.4783 & 0.4788 $\pm$ 0.0001 & 0.4831 $\pm$ 0.0111 \\
$2$    & 0.5166 & 0.3581 $\pm$ 0.0001 & 0.3603 $\pm$ 0.0087 \\
$4$    & 0.5441 & 0.2297 $\pm$ 0.0001 & 0.2299 $\pm$ 0.0093 \\
$8$    & 0.5702 & 0.1731 $\pm$ 0.0001 & 0.1551 $\pm$ 0.0053 \\
$16$   & 0.5947 & 0.1712 $\pm$ 0.0001 & 0.1462 $\pm$ 0.0016 \\
$32$   & 0.6177 & 0.2637 $\pm$ 0.0002 & 0.1462 $\pm$ 0.0020 \\
$64$   & 0.6355 & 0.2176 $\pm$ 0.0001 & 0.1519 $\pm$ 0.0037 \\
\bottomrule
\end{tabular}
\end{sc}
\end{small}
\end{center}
\vskip -0.1in
\end{table}

\todo{Take-away: Talk about how label DP isn't sufficient. One can be adaptive and learn ``through'' the label DP by figuring out how to better group events before adding noise.

Note that we almost optimize the loss perfectly compared to without having label DP.
This can be explained if we have an optimal prior $\th^*$ and large enough batch size,
since the mean will be ``perfect'' but now we've reduced $\eps$ by a factor of $k$.
This suggests larger batch sizes only help once we have a good prior!

Note that taking prefix isn't as good for DP because we know that RRE doesn't converge as nicely.

As final plot shows, it's not enough to simply increase bag size with DP (clearly worse as we increase $k$ for random partitions). Instead, we need a method for forming consistent bags w.r.t. the true response, which is where \PriorBoost comes in. Then once we have these
bags, we can add less DP noise and hence achieve better test performance for a fixed value of $\varepsilon$!
}

\subsection{Application to recommender systems}

\todo{
\begin{itemize}
    %\item Is there a bag size $m$ such that after DP, we do better than $m=1$.
    \item Real world data: Criteo, other recommender systems?
    \item ``Transfer bagging:'' $y' = f(Ux) + \epsilon$ and $y = g(Ux) + \epsilon$,
    where we have all labels $y'$
\end{itemize}
}
